# Supplementary material for: Digital Platform Consolidation and Offline Expansion: Strategic Convergence and Market Welfare in China's Second-hand Real Estate Market
Source: arXiv:2409.04326 source file (2025-04-21)
Supplement: Supplementary file 1 [file other_indices_appendix.tex]

\textbf{Panel A: max(closeness centrality)}\\
\begin{tabular}{lrrrrrll}
\hline
 city      &   2016 &   2017 &   2018 &   2019 &   2020 & 2021   & 2022   \\
\hline
 Beijing   & 0.0174 & 0.0259 & 0.0315 & 0.0338 & 0.035  &        &        \\
 Chengdu   & 0.1365 & 0.2231 & 0.2291 & 0.2675 & 0.282  &        &        \\
 Chongqing & 0.029  & 0.0469 & 0.0483 & 0.0543 & 0.0986 & 0.1006 & 0.0986 \\
 Guangzhou & 0.0317 & 0.0289 & 0.0359 & 0.0357 & 0.0308 & 0.1021 & 0.0932 \\
 Hangzhou  & 0.0556 & 0.0791 & 0.0652 & 0.0584 & 0.085  & 0.0527 & 0.0650 \\
 Nanjing   & 0.0493 & 0.1133 & 0.0868 & 0.1626 & 0.2083 & 0.2073 & 0.1841 \\
 Shanghai  & 0.1132 & 0.0682 & 0.0835 & 0.1024 & 0.0449 & 0.0944 & 0.0376 \\
 Shenzhen  & 0.0362 & 0.0453 & 0.0485 & 0.0379 & 0.0863 &        &        \\
 Tianjin   & 0.0481 & 0.0407 & 0.0371 & 0.0961 & 0.1688 & 0.1837 & 0.1838 \\
 Wuhan     & 0.0259 & 0.0509 & 0.0491 & 0.0357 & 0.0642 &        &        \\
\hline
\end{tabular}

\textbf{Panel B: mean(closeness centrality)}\\
\begin{tabular}{lrrrrrll}
\hline
 city      &   2016 &   2017 &   2018 &   2019 &   2020 & 2021   & 2022   \\
\hline
 Beijing   & 0.0015 & 0.0024 & 0.0025 & 0.0023 & 0.0031 &        &        \\
 Chengdu   & 0.015  & 0.032  & 0.0336 & 0.042  & 0.0415 &        &        \\
 Chongqing & 0.0031 & 0.0036 & 0.0039 & 0.0036 & 0.0073 & 0.0071 & 0.0070 \\
 Guangzhou & 0.0031 & 0.0034 & 0.0029 & 0.0038 & 0.0026 & 0.0079 & 0.0071 \\
 Hangzhou  & 0.0056 & 0.0076 & 0.0055 & 0.0047 & 0.0068 & 0.0039 & 0.0042 \\
 Shenzhen  & 0.003  & 0.0042 & 0.0042 & 0.0039 & 0.0079 &        &        \\
 Shanghai  & 0.0089 & 0.0045 & 0.0064 & 0.0071 & 0.0032 & 0.0060 & 0.0028 \\
 Tianjin   & 0.0053 & 0.0045 & 0.0041 & 0.0071 & 0.0146 & 0.0165 & 0.0164 \\
 Wuhan     & 0.0028 & 0.0039 & 0.003  & 0.0027 & 0.0058 &        &        \\
 Nanjing   & 0.0045 & 0.0113 & 0.008  & 0.0158 & 0.0229 & 0.0202 & 0.0166 \\
\hline
\end{tabular}

\textbf{Panel C: median(closeness centrality)}\\
\begin{tabular}{lrrrrrll}
\hline
 city      &   2016 &   2017 &   2018 &   2019 &   2020 & 2021   & 2022   \\
\hline
 Guangzhou & 0.0003 & 0.0002 & 0.0002 & 0.0002 & 0.0001 & 0.0001 & 0.0001 \\
 Beijing   & 0.0001 & 0      & 0      & 0      & 0      &        &        \\
 Chengdu   & 0.0001 & 0.0001 & 0.0001 & 0      & 0      &        &        \\
 Chongqing & 0.0003 & 0.0002 & 0.0002 & 0.0001 & 0.0001 & 0.0001 & 0.0001 \\
 Hangzhou  & 0.0003 & 0.0002 & 0.0002 & 0.0001 & 0.0001 & 0.0001 & 0.0001 \\
 Shenzhen  & 0.0002 & 0.0001 & 0.0001 & 0.0001 & 0.0001 &        &        \\
 Shanghai  & 0      & 0      & 0      & 0      & 0      & 0.0000 & 0.0000 \\
 Tianjin   & 0.0001 & 0.0001 & 0.0001 & 0.0001 & 0.0001 & 0.0001 & 0.0001 \\
 Wuhan     & 0.0004 & 0.0002 & 0.0002 & 0.0001 & 0.0001 &        &        \\
 Nanjing   & 0.0002 & 0.0001 & 0.0001 & 0.0001 & 0.0001 & 0.0001 & 0.0001 \\
\hline
\end{tabular}

\textbf{Panel D: max(degree centrality)}\\
\begin{tabular}{lrrrrrll}
\hline
 city      &   2016 &   2017 &   2018 &   2019 &   2020 & 2021   & 2022   \\
\hline
 Beijing   & 0.0029 & 0.0026 & 0.0027 & 0.0026 & 0.0025 &        &        \\
 Chengdu   & 0.0075 & 0.0064 & 0.0063 & 0.0055 & 0.0061 &        &        \\
 Chongqing & 0.0118 & 0.0121 & 0.0098 & 0.0067 & 0.0052 & 0.0052 & 0.0051 \\
 Guangzhou & 0.0207 & 0.0096 & 0.0121 & 0.0101 & 0.006  & 0.0060 & 0.0061 \\
 Hangzhou  & 0.0126 & 0.0096 & 0.0095 & 0.0079 & 0.0076 & 0.0060 & 0.0065 \\
 Shanghai  & 0.0045 & 0.0034 & 0.0033 & 0.0038 & 0.0038 & 0.0034 & 0.0036 \\
 Shenzhen  & 0.0084 & 0.0076 & 0.0078 & 0.0081 & 0.0075 &        &        \\
 Tianjin   & 0.0092 & 0.0081 & 0.0074 & 0.007  & 0.0079 & 0.0092 & 0.0093 \\
 Wuhan     & 0.0141 & 0.0119 & 0.0105 & 0.0082 & 0.0064 &        &        \\
 Nanjing   & 0.0078 & 0.0071 & 0.0077 & 0.0074 & 0.0069 & 0.0069 & 0.0073 \\
\hline
\end{tabular}

\textbf{Panel E: mean(degree centrality)}\\
\begin{tabular}{lrrrrrll}
\hline
 city      &   2016 &   2017 &   2018 &   2019 &   2020 & 2021   & 2022   \\
\hline
 Shanghai  & 0.0002 & 0.0002 & 0.0002 & 0.0002 & 0.0002 & 0.0002 & 0.0002 \\
 Wuhan     & 0.0009 & 0.0007 & 0.0007 & 0.0005 & 0.0005 &        &        \\
 Tianjin   & 0.0004 & 0.0005 & 0.0004 & 0.0004 & 0.0004 & 0.0005 & 0.0005 \\
 Shenzhen  & 0.0005 & 0.0006 & 0.0005 & 0.0005 & 0.0005 &        &        \\
 Nanjing   & 0.0005 & 0.0006 & 0.0006 & 0.0005 & 0.0005 & 0.0005 & 0.0005 \\
 Hangzhou  & 0.0008 & 0.0006 & 0.0006 & 0.0005 & 0.0005 & 0.0005 & 0.0005 \\
 Guangzhou & 0.0007 & 0.0006 & 0.0007 & 0.0007 & 0.0004 & 0.0005 & 0.0005 \\
 Chongqing & 0.0007 & 0.0007 & 0.0006 & 0.0004 & 0.0004 & 0.0004 & 0.0004 \\
 Chengdu   & 0.0003 & 0.0003 & 0.0003 & 0.0003 & 0.0002 &        &        \\
 Beijing   & 0.0002 & 0.0002 & 0.0002 & 0.0002 & 0.0002 &        &        \\
\hline
\end{tabular}

\textbf{Panel F: median(degree centrality)}\\
\begin{tabular}{lrrrrrll}
\hline
 city      &   2016 &   2017 &   2018 &   2019 &   2020 & 2021   & 2022   \\
\hline
 Beijing   & 0.0001 & 0      & 0      & 0      & 0      &        &        \\
 Chengdu   & 0.0001 & 0.0001 & 0.0001 & 0      & 0      &        &        \\
 Chongqing & 0.0003 & 0.0002 & 0.0002 & 0.0001 & 0.0001 & 0.0001 & 0.0001 \\
 Guangzhou & 0.0003 & 0.0002 & 0.0002 & 0.0002 & 0.0001 & 0.0001 & 0.0001 \\
 Hangzhou  & 0.0003 & 0.0002 & 0.0002 & 0.0001 & 0.0001 & 0.0001 & 0.0001 \\
 Nanjing   & 0.0002 & 0.0001 & 0.0001 & 0.0001 & 0.0001 & 0.0001 & 0.0001 \\
 Shanghai  & 0      & 0      & 0      & 0      & 0      & 0.0000 & 0.0000 \\
 Shenzhen  & 0.0002 & 0.0001 & 0.0001 & 0.0001 & 0.0001 &        &        \\
 Tianjin   & 0.0001 & 0.0001 & 0.0001 & 0.0001 & 0.0001 & 0.0001 & 0.0001 \\
 Wuhan     & 0.0004 & 0.0002 & 0.0002 & 0.0001 & 0.0001 &        &        \\
\hline
\end{tabular}

\textbf{Panel G: max(page rank)}\\
\begin{tabular}{lrrrrrll}
\hline
 city      &   2016 &   2017 &   2018 &   2019 &   2020 & 2021   & 2022   \\
\hline
 Beijing   & 0.0014 & 0.0011 & 0.0011 & 0.001  & 0.0007 &        &        \\
 Chengdu   & 0.0036 & 0.0025 & 0.0021 & 0.0018 & 0.0011 &        &        \\
 Guangzhou & 0.0102 & 0.0041 & 0.0042 & 0.0059 & 0.0024 & 0.0012 & 0.0011 \\
 Hangzhou  & 0.0067 & 0.0042 & 0.0034 & 0.0042 & 0.0016 & 0.0015 & 0.0016 \\
 Chongqing & 0.0085 & 0.0069 & 0.0045 & 0.0034 & 0.0019 & 0.0014 & 0.0011 \\
 Shanghai  & 0.0011 & 0.0013 & 0.001  & 0.0008 & 0.001  & 0.0018 & 0.0013 \\
 Shenzhen  & 0.0046 & 0.0023 & 0.0024 & 0.0037 & 0.0012 &        &        \\
 Tianjin   & 0.0048 & 0.0038 & 0.0052 & 0.0043 & 0.0021 & 0.0017 & 0.0016 \\
 Wuhan     & 0.0085 & 0.0044 & 0.0032 & 0.0031 & 0.0011 &        &        \\
 Nanjing   & 0.005  & 0.0022 & 0.0024 & 0.0023 & 0.0016 & 0.0014 & 0.0011 \\
\hline
\end{tabular}

\textbf{Panel H: mean(page rank)}\\
\begin{tabular}{lrrrrrll}
\hline
 city      &   2016 &   2017 &   2018 &   2019 &   2020 & 2021   & 2022   \\
\hline
 Beijing   & 0.0001 & 0.0001 & 0.0001 & 0.0001 & 0.0001 &        &        \\
 Chengdu   & 0.0001 & 0.0001 & 0.0001 & 0.0001 & 0.0001 &        &        \\
 Guangzhou & 0.0007 & 0.0003 & 0.0004 & 0.0004 & 0.0002 & 0.0001 & 0.0001 \\
 Hangzhou  & 0.0005 & 0.0004 & 0.0004 & 0.0003 & 0.0002 & 0.0002 & 0.0002 \\
 Chongqing & 0.0006 & 0.0005 & 0.0004 & 0.0003 & 0.0002 & 0.0001 & 0.0001 \\
 Shanghai  & 0.0001 & 0.0001 & 0.0001 & 0.0001 & 0.0001 & 0.0001 & 0.0001 \\
 Shenzhen  & 0.0003 & 0.0003 & 0.0003 & 0.0003 & 0.0002 &        &        \\
 Tianjin   & 0.0003 & 0.0003 & 0.0003 & 0.0002 & 0.0001 & 0.0001 & 0.0001 \\
 Wuhan     & 0.0007 & 0.0004 & 0.0003 & 0.0002 & 0.0001 &        &        \\
 Nanjing   & 0.0003 & 0.0003 & 0.0003 & 0.0002 & 0.0002 & 0.0001 & 0.0001 \\
\hline
\end{tabular}

\textbf{Panel I: median(page rank)}\\
\begin{tabular}{lrrrrrll}
\hline
 city      &   2016 &   2017 &   2018 &   2019 &   2020 & 2021   & 2022   \\
\hline
 Tianjin   & 0.0001 & 0.0001 & 0.0001 & 0.0001 & 0      & 0.0000 & 0.0000 \\
 Beijing   & 0      & 0      & 0      & 0      & 0      &        &        \\
 Chengdu   & 0.0001 & 0      & 0      & 0      & 0      &        &        \\
 Chongqing & 0.0003 & 0.0002 & 0.0001 & 0.0001 & 0.0001 & 0.0000 & 0.0000 \\
 Guangzhou & 0.0003 & 0.0001 & 0.0001 & 0.0002 & 0.0001 & 0.0000 & 0.0000 \\
 Hangzhou  & 0.0002 & 0.0001 & 0.0001 & 0.0001 & 0.0001 & 0.0001 & 0.0001 \\
 Nanjing   & 0.0001 & 0.0001 & 0.0001 & 0.0001 & 0.0001 & 0.0000 & 0.0000 \\
 Shanghai  & 0      & 0      & 0      & 0      & 0      & 0.0000 & 0.0000 \\
 Shenzhen  & 0.0001 & 0.0001 & 0.0001 & 0.0001 & 0.0001 &        &        \\
 Wuhan     & 0.0003 & 0.0001 & 0.0001 & 0.0001 & 0      &        &        \\
\hline
\end{tabular}
